# Supplementary material for: GeoIB: Geometry-Aware Information Bottleneck via Statistical-Manifold Compression
Source: arXiv:2602.03906 source file (2026-02-03)
Supplement: Supplementary file 1 [file appendix2.tex]

\begin{table*}[t]
	% \tiny
	\scriptsize
	\caption{Overall Evaluation Results on MNIST, CIFAR10 and CelebA.	\vspace{-2mm}}
	\label{tab_total}
	\resizebox{\linewidth}{!}{
		\setlength\tabcolsep{2.pt}
		\begin{tabular}{c|cccccccccccc}
			\toprule[1pt]
			\multirow{2}{*} {\makecell[c]{\makecell[c]{\textbf{Single-Sample}\\ \textbf{Unlearning}} }} & \multicolumn{4}{c} {MNIST}& \multicolumn{4}{c} {CIFAR10} & \multicolumn{4}{c} {CelebA}  \\
			\cmidrule(r){2-5}   \cmidrule(r){6-9} \cmidrule(r){10-13}
			& OUbL & BFU   &SISA 	 &VBU 	 &OUbL & BFU  & SISA  & VBU	 & OUbL  & BFU  & SISA  &VBU\\
			\midrule %\thinmidrule
			Model Accuracy &  98.71\% & \textbf{98.88\%}  &{98.75\%}  & 97.91\%      & 76.75\%     & 77.61\%   	  & \textbf{79.37\%}   	&75.86\%   & 95.66\% & 95.72\%	& \textbf{95.78\%} & 95.80\%\\
			Backdoor Accuracy & \textbf{0.00\%}   & \cellcolor{lightred} 100\%	    & \textbf{0.00\%}   & \textbf{0.00\%}   &  0.00\% &  \cellcolor{lightred} 100\%  & 0.00\%&  \textbf{0.00\%}		&0.00\%	 & \cellcolor{lightred}100\%   & \textbf{0.00\%} & 0.00\%  \\
			Unl. Update Similarity 		 	& \textbf{0.976}  	& -  		 &-   	& - 		& \textbf{0.989} &  -	 & - & - 	&\textbf{0.998} & -    &- & - \\
			Reconstruction Similarity     & \textbf{0.669}  &  0.947   & 1  & 1     & \textbf{0.852} & 0.888  &  1 & 1   & \textbf{0.932}  &  0.933 & 1 & 1 \\
			Running time (s)  	  & 4.178  & 15.95  & 11.87		& \textbf{0.024}  		        &8.231   &122.26 &  113.00 		& \textbf{0.088}	 		&0.432 	&168.61 	& 135.42 & \textbf{0.033} \\
			\midrule[0.12em]
			\multirow{2}{*} {\makecell[c]{\makecell[c]{\textbf{Multi-Sample}\\ \textbf{Unlearning}} }} & \multicolumn{4}{c} {MNIST, $\text{\it USR}=1\%$}& \multicolumn{4}{c} {CIFAR10, $\text{\it USR}=1\%$} & \multicolumn{4}{c} {CelebA, $\text{\it USR}=0.5\%$}  \\
			\cmidrule(r){2-5}   \cmidrule(r){6-9} \cmidrule(r){10-13}
			&OUbL & BFU  &SISA	 &VBU	 &OUbL   & BFU & SISA  & VBU		  & OUbL & BFU  & SISA  &VBU\\
			\midrule %\thinmidrule
			Model Accuracy &  98.52\% & \textbf{98.70\%} & {98.53\%}  & 78.69\%     & 73.89\%    & 78.20\%     	  & \textbf{78.49\%}   	&43.23\%  & 95.74\%	& \textbf{96.01\%}  & 95.92\% & 93.53\%\\
			Backdoor Accuracy  	 & 9.67\%   & 9.16\%    & 9.67\%   & \textbf{0.00\%}   &  9.40\%  &  9.70\%	       & 7.60\%&  \textbf{0.00\%} &4.55\%	&\cellcolor{lightred} 41.92\%  & \textbf{4.41\%} & 4.92\%  \\
			Unl. Update Similarity 		 	& \textbf{0.942}  	& -  		 &-   	& - 		& \textbf{0.959} &  -	 & - & - 	&\textbf{0.992} & -    &- & - \\
			Reconstruction Similarity       & \textbf{0.818} &  0.874  & 1  & 1    & \textbf{0.846} & 0.874   &  1 & 1    & \textbf{0.826} &  0.831 & 1 & 1 \\
			Running time (s)  	  & 3.920  & 16.03   & 11.70		& \textbf{0.631}     &6.633  &141.26  &  103.01 		& \textbf{0.587}	 		&{2.257}	&176.86 	& 133.74 & \textbf{0.672} \\
			\bottomrule[1pt]
	\end{tabular}}
	\begin{tabbing}
		\scriptsize % \scriptsize % \footnotesize \small
		BFU \citep{wang2023bfu}; SISA \citep{bourtoule2021machine}; VBU \citep{nguyen2020variational}
	\end{tabbing}
	\vspace{-6mm}
\end{table*}

\section{Additional Experiments} \label{exp_appendix}

\subsection{Overall Evaluation of OUbL} \label{Overall_eva}

% \usepackage{braket} \makecell[c]{}

%58.48
%\cellcolor{lightred}

% In this subsection, we demonstrate the overview evaluation results of different methods on MNIST, CIFAR10 and CelebA, presented in \Cref{tab_total}. 
%The bolded values indicate the best performance among the compared methods, while red-colored values signify results that are opposite from expectations.

We first demonstrate the overall evaluation results of different machine unlearning methods on MNIST, CIFAR10 and CelebA, presented in \Cref{tab_total}. The bolded values indicate the best performance among the compared methods, while red-colored values signify results that are opposite from expectations. We fill a dash when the method does not contain the evaluation metrics.

%\vspace{2mm}
\noindent
\textbf{Setup.} 
We measure unlearning methods based on the five above-introduced evaluation metrics in single-sample and multi-sample unlearning scenarios. In the single samples unlearning scenario, only one unlearning sample needs to be unlearned. In the multi-sample unlearning scenario, we set the unlearning samples rate $\text{\it USR}=1\%$, where $\text{\it USR} = \frac{m}{n}$, $m$ is the unlearned samples size and $n$ is the training data size. We illustrate the comparison of OUbL with one privacy-preserving federated unlearning method, BFU \citep{wang2023bfu}, one representative exact unlearning method, SISA \citep{bourtoule2021machine}, and one approximate unlearning method, VBU \citep{nguyen2020variational}.

%We demonstrate the overview evaluation results of different unlearning methods on MNIST, CIFAR10 and CelebA, presented in \Cref{tab_total}. We measure unlearning methods based on the above-introduced evaluation metrics except for the forgeability, which will be analyzed later. The evaluations is conducted in both single-sample and multi-sample scenarios, where the Erased Samples Size ($ESS$) equal to 1 and 20 respectively. The bolded values indicate the best performance among the compared methods.

%We measure verification methods based on the five above-introduced evaluation metrics in single-sample and multi-sample unlearning scenarios. In single-sample verification, we set the Erased Sample Size ($ESS$) equal to 1 and $ESS=20$ for the multi-sample scenario. We fill a dash when the method does not contain the evaluation metrics. The evaluation of PEDR includes the classifying task (CT) and autoencoding task (AT), $\alpha=0$ and $\alpha=0.9$, respectively. Here, we choose $\alpha=0.9$ rather than $\alpha=1$ (the model only has autoencoder task) because we hope to use the model accuracy still to evaluate the model utility. Although MIB is only suitable for the classifying task, we use the same model structure as PEDR and set $\alpha=0.9$ for the implementation of MIB. 

%We compared our UEV with the state-of-the-art unlearning verification method MIB \cite{hu2022membership}. 

%\vspace{2mm}
\noindent
\textbf{Evaluation of Unlearning Effectiveness.}
The effect of machine unlearning is measured by model accuracy and backdoor accuracy, where the model accuracy represents the model utility after unlearning, and the backdoor accuracy means if the backdoor-marked samples are unlearned from the model. 

From the model utility perspective, in most cases, BFU or SISA achieves the best model accuracy. This is because SISA is a retraining-based method, and BFU needs all other normal federated users to assist in unlearning retraining to ensure the model's utility. Compared with the methods utilizing the remaining dataset, OUbL achieves a similar model accuracy as BFU and SISA, usually only slightly lower (not exceeding 2\%) than them, much better than VBU, an approximate unlearning method without the assistance of the remaining dataset.

From the data removal perspective, OUbL and other centralized unlearning methods (SISA and VBU) can effectively unlearn the marked samples, reducing the backdoor accuracy to a very low level. For BFU, although the retraining assistance of other normal federated users helps to preserve model utility, it to some extent mitigates the unlearning update, failing to unlearn specified samples in the single-sample scenario on all datasets and in the multi-sample scenario on CelebA. 

%sometimes.

\noindent
\textbf{Evaluation of Privacy Protection.}
We evaluate privacy preservation through reconstruction similarity metrics. For OUbL and BFU, since the server cannot access the erased data, we conduct the reconstruction attacks \citep{Hu2024sp,salem2020updates,zhang2023conditional} based on the unlearned update. Since the server of OUbL has no information about unlearning intentions, it treats the model updates as normal learning updates for attack \citep{salem2020updates}. 

The results of the three datasets show significant improvement in privacy protection by hiding unlearning intentions. For example, on MNIST, for SISA and VBU, since the server knows the unlearning requested samples, the reconstruction similarity is directly 1, the same as having no privacy preservation of these data. When gradient-based protection (BFU) is applied, the privacy protection of erased data achieves 0.947 reconstruction similarity when unlearning one sample. If we inform the server with unlearning intentions in OUbL, it achieves a reconstruction similarity to BFU. We present detailed comparisons for OUbL with informed unlearning intentions in \Cref{impact_of_unl_intentions}. However, the server will be oblivious to unlearning when conducting OUbL, and the privacy protection of OUbL achieves 0.669 reconstruction similarity on single-sample unlearning on MNIST. OUbL achieves significant privacy protection on the three datasets compared with the FL-based and no-privacy protection unlearning methods. Although the FL-based method can also protect the privacy of erased data, it sometimes fails to unlearn samples and is inefficient as it needs the retraining assistance of other normal users. 

%We omit the demonstration of privacy preservation of unlearning intentions in \Cref{tab_total} as only OUbL can achieve an unlearning effect without the need for additional algorithms besides the original learning algorithm. We demonstrate the privacy preservation of erased data measured by the reconstruction similarity metric. Since the reconstruction attack is conducted based on the final unlearning model difference, our method achieves privacy protection similar to that of the federated unlearning method, BFU. In SISA and VBU, since the server knows the unlearning requested samples, the reconstruction similarity is directly 1, the same as having no privacy preservation of these data. We should explain that the real erased data privacy preservation of OUbL is much better than demonstrated because the server will not know the update is for unlearning in OUbL. Without this information for attacking, then if we only compare the similarity between the uploaded constructed data with the truly unlearned samples, the similarity would be almost 0.

\noindent
\textbf{Evaluation of Efficiency.}
Normally, OUbL achieves a slight efficiency improvement than BFU and SISA on MNIST and a significant improvement (more than $10 \times$ speedup) on CIFAR10 and CelebA. Although BFU and SISA are much more efficient than naive retraining, they are still training time expensive compared with OUbL and VBU because BFU needs the retraining assistance of other users, and SISA needs to retrain $1/5$ shard of the original training dataset. VBU is the most efficient method, with less than 0.1 seconds for single sample unlearning, as it implements unlearning only based on the erased samples; however, the cost is the model utility degradation and lack of privacy protection.

%OUbL achieves a significant efficiency improvement on CIFAR10 and CelebA than BFU and SISA

\iffalse
\begin{tcolorbox}[colback=white, boxrule=0.3mm]
	\noindent \textbf{Takeaway 1.} By hiding the unlearning intentions from the server, OUbL achieves much better privacy protection than FL-based and no-privacy protection methods, with only a little utility and efficiency compromise.
\end{tcolorbox}
\fi 

% compared to the state-of-the-art no-privacy protection method

%	Unlearning inversion attacks are effective in machine unlearning. For approximate unlearning, the attack can recover the feature as well as the label information of the unlearned data. For exact unlearning, the attack is effective for label inference but is less effective in feature recovery.
% , a little worse than the representative method SISA.

\subsection{Additional Evaluation of Impact of Unlearning Samples Rate ($\text{\it USR}$)} \label{impact_of_USR}

% \noindent
%\textbf{Impact of Unlearning Samples}
%This is the size introduced in \cite{thudi2022necessity}, larger size of unlearning samples makes forging eaiser.

\begin{figure*}[t]
	\centering
	\hspace{-5mm}
	\subfloat{ 	\label{fig:mnistforgeabilityurs} \rotatebox{90}{ \hspace{8mm}	\scriptsize{ On MNIST} }
		\includegraphics[scale=0.19]{../../../../PycharmProjects/OUL/Experimental_results/On_MNIST/Forgeability/mnist_forgeability_urs}
	}			
	\hspace{-3mm}
	\subfloat{  	 	\label{fig:mnistmodelaccurs} 
		\includegraphics[scale=0.19]{../../../../PycharmProjects/OUL/Experimental_results/On_MNIST/Model_acc/mnist_model_acc_urs}
	} 
	\hspace{-3mm}
	\subfloat{ \label{fig:mnistbackaccurs}
		\includegraphics[scale=0.19]{../../../../PycharmProjects/OUL/Experimental_results/On_MNIST/Back_acc/mnist_back_acc_urs}
	}
	\hspace{-3mm}
	\subfloat{   	\label{fig:mnistreconsimurs}
		\includegraphics[scale=0.19]{../../../../PycharmProjects/OUL/Experimental_results/On_MNIST/Recon_sim/mnist_recon_sim_urs}
	}
	\hspace{-3mm}
	\subfloat{ 	 	\label{fig:mnistrunningtimeurs} 
		\includegraphics[scale=0.19]{../../../../PycharmProjects/OUL/Experimental_results/On_MNIST/Running_time/mnist_running_time_urs}
	} \vspace{-3mm} \\
	\hspace{-5mm}
	\subfloat{  	\label{fig:cifar10forgeabilityurs}  \rotatebox{90}{ \hspace{8mm}	\scriptsize{ On CIFAR10} }
		\includegraphics[scale=0.19]{../../../../PycharmProjects/OUL/Experimental_results/On_CIFAR10/Forgeability/cifar10_forgeability_urs}
	} 
	\hspace{-3mm}
	\subfloat{ 	 	\label{fig:cifar10modelaccurs}
		\includegraphics[scale=0.19]{../../../../PycharmProjects/OUL/Experimental_results/On_CIFAR10/Model_acc/cifar10_model_acc_urs}
	}			
	\hspace{-3mm}
	\subfloat{ 	\label{fig:cifar10backaccurs}
		\includegraphics[scale=0.19]{../../../../PycharmProjects/OUL/Experimental_results/On_CIFAR10/Back_acc/cifar10_back_acc_urs}
	}
	\hspace{-3mm}
	\subfloat{    	\label{fig:cifar10reconsimurs}
		\includegraphics[scale=0.19]{../../../../PycharmProjects/OUL/Experimental_results/On_CIFAR10/Recon_sim/cifar10_recon_sim_urs}
	}
	\hspace{-3mm}
	\subfloat{  	\label{fig:cifar10runningtimeurs}
		\includegraphics[scale=0.19]{../../../../PycharmProjects/OUL/Experimental_results/On_CIFAR10/Running_time/cifar10_running_time_urs}
	} \vspace{-3mm}  
	\caption{Evaluations of impact about different $\text{\it USR}$. \vspace{-0mm} } %\vspace{-2mm}
	\label{evaluation_of_USR} 
	\vspace{-4mm}
\end{figure*}

\noindent
\textbf{Setup.} 
Since the above unlearning methods have lots of similar metric values, for clear illustration and demonstration, we here only display the VBU and VBU-LDP methods as they implement machine unlearning based on solely erased samples, which requires the least data access. In this experiment, we range $\text{\it USR}$ from 1\% to 6\% on MNIST and CIFAR10. %, from 0.5\% to 1\% on CelebA. 
$\text{\it CSR}$ and $\text{\it ASR}$ are set 1\% for OUbL on MNIST and CIFAR10. %, and 0.5\% for OUbL on CelebA. 
The privacy budget of VBU-LDP is set $\epsilon=10$ here. All the experimental results are presented in \Cref{evaluation_of_USR}.

\noindent
\textbf{Relationship between Unlearning Update Similarity and $\text{\it USR}$.}
The first column of \Cref{evaluation_of_USR} shows the relationship between unlearning update similarity and $\text{\it USR}$. It is obvious that more unlearning samples in the unlearning request will increase the difficulty of constructing the dataset to achieve the unlearning effect, which is confirmed on the three datasets, higher $\text{\it USR}$ decreasing the unlearning update similarity of OUbL a lot.

\noindent
\textbf{Impact on Unlearning Effectiveness.}
Unlearning effectiveness includes model utility preservation (the second column) and the data removal effect (the third column) in \Cref{evaluation_of_USR}. 

From the model utility preservation perspective, a good unlearning method should not be heavily influenced by the increasing $\text{\it USR}$. On all datasets, OUbL always achieves a similar model accuracy as the original trained model on all datasets even when $\text{\it USR}$ increases from 1\% to 6\%. VBU only achieves an acceptable model accuracy on CelebA. Moreover, adding the LDP noise will definitely decrease the model utility, reflected by the huge gap between VBU and VBU-LDP.

From the data removal perspective, all the unlearning methods can effectively remove the influence of the marked backdooring samples from the model, reducing the backdoor accuracy of the original model. %Although VBU achieves a thorough data removal effect, which is better than OUbL, we also note that the noise injection will mitigate the data removal effect, as shown in the third figure on CelebA.

\noindent
\textbf{Impact on Erased Data Protection.} 
The fourth column in \Cref{evaluation_of_USR} shows the privacy protection of the erased samples against the reconstruction attacks \citep{Hu2024sp,zhang2023conditional}. For these methods with no privacy protection, the server directly has the erased sample, and the reconstruction similarity is 1. When $\text{\it USR}$ increases, the reconstruction similarity of OUbL increases, too, meaning more privacy is leaked. Since we set $\epsilon=10$ for VBU-LDP, OUbL always achieves better privacy protection than VBU-LDP.

%The fourth column in \Cref{evaluation_of_USR} shows the privacy protection of the erased samples against the reconstruction attacks \citep{Hu2024sp,zhang2023conditional}. Even if we assume that we expose the unlearning intention information to the adversary server in OUbL, we still achieve much better privacy protection than LDP protection ($\epsilon=10$, VBU-LDP) against the reconstruction attacks. As $\text{\it USR}$ increases, the privacy protection of OUbL increases, showing lower reconstructed similarity in the fourth column in \Cref{evaluation_of_USR}.

\noindent
\textbf{Impact on Unlearning Efficiency.} 
The fifth column in \Cref{evaluation_of_USR} illustrates the running time of OUbL and VBU. 
The running time slightly increases as $\text{ \it USR}$ increases. Both OUbL and VBU achieve more than $20 \times$ speedup than original training, which is much more efficient than most federated unlearning and retraining-based methods. Although OUbL consumes slightly more time than VBU, it is important to note that OUbL does not require uploading the erased data and informing the server for unlearning, which avoids privacy leakage of both erased data and unlearning intentions. 

\iffalse
\begin{tcolorbox}[colback=white, boxrule=0.3mm]
	\noindent \textbf{Takeaway 4.} More unlearning samples reduce the unlearning update similarity of OUbL when synthesizing the new dataset. However, OUbL still achieves stable unlearning effectiveness, slight privacy protection and efficiency decrease when $\text{\it USR}$ increases. 
\end{tcolorbox}
\fi

\begin{figure*}[h]
	\centering
	\hspace{-5mm}
	\subfloat{ 	\label{fig:mnistorgsimnoiseanalysis}  \rotatebox{90}{ \hspace{8mm}	\scriptsize{ On MNIST} }
		\includegraphics[scale=0.19]{../../../../PycharmProjects/OUL/Experimental_results/On_MNIST/Original_sim/mnist_org_sim_noise_analysis}
	}			
	\hspace{-3mm}
	\subfloat{  \label{fig:mnistforgeabilityunlsim}
		\includegraphics[scale=0.19]{../../../../PycharmProjects/OUL/Experimental_results/On_MNIST/Forgeability/mnist_forgeability_unl_sim}
	} 
	\hspace{-3mm}
	\subfloat{\label{fig:mnistmodelaccunlsim}  
		\includegraphics[scale=0.19]{../../../../PycharmProjects/OUL/Experimental_results/On_MNIST/Model_acc/mnist_model_acc_unl_sim}
	}			
	\hspace{-3mm}
	\subfloat{ 		\label{fig:mnistbackaccunlsim}
		\includegraphics[scale=0.19]{../../../../PycharmProjects/OUL/Experimental_results/On_MNIST/Back_acc/mnist_back_acc_unl_sim}
	}
	\hspace{-3mm}
	\subfloat{  		\label{fig:mnistreconsimunlsim}
		\includegraphics[scale=0.19]{../../../../PycharmProjects/OUL/Experimental_results/On_MNIST/Recon_sim/mnist_recon_sim_unl_sim}
	}\vspace{-3mm} \\
	\hspace{-5mm}
	\subfloat{ 	  	\label{fig:cifar10orgsimnoiseanalysis} \rotatebox{90}{ \hspace{8mm}	\scriptsize{ On CIFAR10} }
		\includegraphics[scale=0.19]{../../../../PycharmProjects/OUL/Experimental_results/On_CIFAR10/Original_sim/cifar10_org_sim_noise_analysis}
	}			
	\hspace{-3mm}
	\subfloat{  \label{fig:cifar10forgeabilityunlsim}
		\includegraphics[scale=0.19]{../../../../PycharmProjects/OUL/Experimental_results/On_CIFAR10/Forgeability/cifar10_forgeability_unl_sim}
	} 
	\hspace{-3mm}
	\subfloat{ 	 	\label{fig:cifar10modelaccunlsim}  
		\includegraphics[scale=0.19]{../../../../PycharmProjects/OUL/Experimental_results/On_CIFAR10/Model_acc/cifar10_model_acc_unl_sim}
	}			
	\hspace{-3mm}
	\subfloat{ 	 	\label{fig:cifar10backaccunlsim}
		\includegraphics[scale=0.19]{../../../../PycharmProjects/OUL/Experimental_results/On_CIFAR10/Back_acc/cifar10_back_acc_unl_sim}
	}
	\hspace{-3mm}
	\subfloat{    	\label{fig:cifar10reconsimunlsim}
		\includegraphics[scale=0.19]{../../../../PycharmProjects/OUL/Experimental_results/On_CIFAR10/Recon_sim/cifar10_recon_sim_unl_sim}
	} \vspace{-3mm}  \\
	\hspace{-5mm}
	\subfloat{		\label{fig:celebaorgsimnoiseanalysis} \rotatebox{90}{ \hspace{8mm}	\scriptsize{ On CelebA} }
		\includegraphics[scale=0.19]{../../../../PycharmProjects/OUL/Experimental_results/On_CelebA/Original_sim/celebA_org_sim_noise_analysis}
	}	
	\hspace{-3mm}
	\subfloat{ 	\label{fig:celebaforgeabilityunlsim}
		\includegraphics[scale=0.19]{../../../../PycharmProjects/OUL/Experimental_results/On_CelebA/Forgeability/CelebA_forgeability_unl_sim}
	} 		
	\hspace{-3mm}
	\subfloat{	\label{fig:celebamodelaccunlsim}  
		\includegraphics[scale=0.19]{../../../../PycharmProjects/OUL/Experimental_results/On_CelebA/Model_acc/CelebA_model_acc_unl_sim}
	}			
	\hspace{-3mm}
	\subfloat{ 		\label{fig:celebabackaccunlsim}
		\includegraphics[scale=0.19]{../../../../PycharmProjects/OUL/Experimental_results/On_CelebA/Back_acc/CelebA_back_acc_unl_sim}
	}
	\hspace{-3mm}
	\subfloat{  		\label{fig:celebareconsimunlsim}
		\includegraphics[scale=0.19]{../../../../PycharmProjects/OUL/Experimental_results/On_CelebA/Recon_sim/CelebA_recon_sim_unl_sim}
	}%\vspace{-2mm}
	\caption{Evaluations for the impact of unlearning samples' similarity} %\vspace{-2mm}
	\label{evaluation_of_unl_sim} 
\end{figure*}

\subsection{Impact of Unlearning Samples Similarity} \label{additional_ablation}

%\noindent
%\textbf{Impact of Unlearning Samples Similarity}

We know that the similarity between the erased samples and the remaining samples plays an important role in machine unlearning. In this section, we also conduct experiments to evaluate how the similarity influences the performance of OUbL.

\vspace{2mm}
\noindent
\textbf{Setup.} To quantify the similarity between the erased samples and the remaining samples, we introduce a backdoor ratio $\beta$ to control the injected patch to the erased samples, formulated as $D_{u, \beta} \gets (X_u + \beta \times patch, Y_u)$. We mixed both $D_{u,\beta}$ and original unlearned data $D_u$ into the training dataset for ML service model training. During the unlearning process, we only need to remove the contribution of the marked samples $D_{u, \beta}$. By adjusting $\beta$, we can simulate the different levels of similarity between the erased samples and the samples in the remaining dataset. This approach allows us to intuitively quantify the similarity between the unlearned samples and the remaining samples. The experimental results on MNIST, CIFAR10 and CelebA are presented in \Cref{evaluation_of_unl_sim}. 

\vspace{1mm}
\noindent
\textbf{Relationship between Unlearned Data Similarity and Patch Injection Ratio.} The first column in \Cref{evaluation_of_unl_sim} illustrates the relationship between the patch injection ratio $\beta$ and similarity, where similarity is measured between the original samples $D_u$ and the patch-injected data $D_{u, \beta}$. In this experiment, we only need to unlearn $D_{u\beta}$. Across all datasets, including MNIST, CIFAR10, and CelebA, increasing the amount of noise (as indicated by a higher $\beta$) results in a decrease in similarity. This trend is consistently observed, demonstrating that higher patch injection ratios make the unlearned samples more distinct from the original samples in the remaining dataset.

\vspace{1mm}
\noindent
\textbf{Impact on Unlearning Update Similarity.}
The second column in \Cref{evaluation_of_unl_sim} demonstrates the unlearning update similarity influenced by the patch ratio $\beta$. With more patches injected into the data, the marked samples will be more dissimilar to the original samples and the remaining samples. It increases the difficulty of OUbL in approaching the unlearning update via incremental learning, as the normal clean and the auxiliary data that we can use are not similar to the unlearned samples with a high patch injecting ratio. The unlearning update similarity obviously decreases as the patch ratio increases on all three datasets.

\vspace{1mm}
\noindent
\textbf{Impact on Unlearning Effectiveness.}
The third and fourth columns demonstrate the model utility and data removal of unlearning effectiveness. The data removal effect increases as the patch ratio increases, showing as the decreased backdoor accuracy. It means the more unique samples, larger $\beta$ and lower similarity, are easier to be unlearned. However, better data removal effect slightly decreases model utility, as showing from the model accuracy of all methods in the third column in \Cref{evaluation_of_unl_sim}.

\vspace{1mm}
\noindent
\textbf{Impact on Erased Data Protection.}
Our OUbL achieves the best privacy protection for the erased samples, and the attacking difficulty for OUbL increases as the patch ratio increases. It is easy to understand because OUbL is more difficult to forge the unlearning update when patch ratio increases, which means the constructed data contains less unqiue information about the erased samples when $\beta$ is large. It makes the unlearning update less similar to the expected ones, and hence increase the reconstruction difficulty.

We omit the illustration of the unlearning efficiency results as the similarity not heavily influence the training time.

%\noindent
%\textbf{Impact on Unlearning Efficiency.}

\iffalse
\begin{tcolorbox}[colback=white, boxrule=0.3mm]
	\noindent \textbf{Takeaway 6.}  As the patch ratio increases, the similarity between the unlearned samples and the remaining dataset decreases, making the unlearned samples more unique. Consequently, OUbL finds it more challenging to approach the unlearning update with a higher patch ratio, which reduces the model's utility to some extent. At the same time, this increased uniqueness makes the model harder to be attacked by reconstruction attacks. 
\end{tcolorbox}
\fi

 \subsection{Impact of Constructed Samples Rate and Auxiliary Samples Rate on Unlearning Efficiency} \label{impact_of_samples_rate_on_eff}

\begin{figure}[h] %{r}{0.52\textwidth}
	\centering
	\vspace{-4mm}
	\includegraphics[width=0.7\linewidth]{../../../../PycharmProjects/OUL/Experimental_results/On_MNIST/Running_time/mnist_running_time_cs_as_bar}
	\caption{The impact of $\text{\it CSR}$ and $\text{\it ASR}$ about the running time. The $\text{\it CSR}$ and $\text{\it ASR}$ for CelebA is from 0.5\% to 1\%. \vspace{-4mm}}
	\label{fig_mnistrunningtimecsasbar}
\end{figure}

%\noindent
\textbf{Impact on Unlearning Efficiency.}
As the synthesized dataset is constructed with the parameters $\text{\it CSR}$ and $\text{\it ASR}$, the incremental training time based on the constructed dataset will definitely increase linearly as $\text{\it CSR}$ and $\text{\it ASR}$ increases, as shown in \Cref{fig_mnistrunningtimecsasbar}.

\clearpage
\newpage

\setcounter{figure}{0}

\begin{figure}
	\centering
	\subfloat{ 	\label{Original_MNIST} 
		\includegraphics[width=0.4\textwidth]{Original_MNIST}
	}		
	\subfloat{ 	\label{Original_cifar10} 
		\includegraphics[width=0.422\textwidth]{Original_cifar10}
	} \\
	\vspace{-3mm}
	\subfloat{ 	\label{OUbL_mnist} 
		\includegraphics[width=0.4\textwidth]{OUbL_mnist}
	}			
	\subfloat{ 	\label{OubL_cifar10} 
		\includegraphics[width=0.422\textwidth]{OubL_cifar10}
	}	\\
	\vspace{-3mm}
	\subfloat{ 	\label{Nose_mnist} 
		\includegraphics[width=0.4\textwidth]{Nose_mnist}
	}			
	\subfloat{ 	\label{Noise_Cifar101} 
		\includegraphics[width=0.422\textwidth]{Noise_Cifar10}
	}	
	\caption{Example of the original auxiliary dataset (the first row), their noisy counterparts (the middle row), and directly construct data without an auxiliary dataset [R11] (the last row). @{\color{red}Reviewer iCGz} } %\vspace{-2mm}
	\label{fig:noisecifar10}
\end{figure}

 % Use R prefix
\setcounter{table}{0}

\begin{table}[H]
	\scriptsize
	\caption{Evaluating mixing unlearned data in the clean dataset on CIFAR10. The results demonstrate that mixing the unlearned samples into the constructed uploaded data for incremental learning negatively impacts the unlearning effect, as reflected by the increasing backdoor accuracy, but the model utility keeps. @{\color{blue}Reviewer BZGC}}
	\label{Evaluating_mixing}
	\resizebox{\linewidth}{!}{
		\setlength\tabcolsep{7.5pt}
		\begin{tabular}{c|c|c|c|c|c}
			\toprule[0.8pt]
			\midrule
			On CIFAR10 & Mixed 0\% of Unlearned Data  & 2\% & 4\% & 6\% & 8\% \\
			\midrule
			Model Acc.      & 73.89\%     & 73.85\%  &  73.78\%  &  73.25\%  &  73.03\%   \\  
			\rowcolor{verylightgray}
			Backdoor Acc.    & 9.40\%       & 13.60\%   & 33.40\%   &  35.40\%   &  43.26\%   \\  
			Running Time     &  6.63        &  6.72     &  6.83     &  7.01     &  7.16  \\
			\midrule
			\bottomrule[0.8pt]
	\end{tabular}}
\end{table}

\begin{table}[H]
	\scriptsize
	\caption{Evaluating learning rate on MNIST and CIFAR10. The results demonstrate that a larger learning rate can speed the convergence to achieve unlearning, costing less computation and achieving a better unlearning effect (low backdoor accuracy by removing). The tradeoff is that it slightly decreases the model utility at the same time, which is not too much on MNIST but a little worse on CIFAR10. @{\color{red}Reviewer iCGz}, @{\color{cyan} Reviewer Gp18}}
	\label{Evaluating_lr}
	\resizebox{\linewidth}{!}{
		\setlength\tabcolsep{7.5pt}
		\begin{tabular}{c|c|c|c|c|c|c}
			\toprule[0.8pt]
			\midrule
			& Metrics & Learning Rate: 0.0001  & 0.0002  & 0.0004 & 0.0006 & 0.0008 \\
			\midrule
			\multirow{3}{*}{\makecell[c]{On MNIST } }  &Model Acc.      & 98.52\%     & 97.84\%   &  96.72\%  &  95.88\%  &  95.37\%    \\  
			\rowcolor{verylightgray}
			On MNIST &Backdoor Acc.    & 9.67\%       & 9.53\%   & 9.17\%   &  8.20\%   &  8.67\%   \\  
			& Running Time     &  3.92        &  2.72     &  1.83     &  1.61     & 1.56   \\
			\midrule
			\multirow{3}{*}{\makecell[c]{On Cifar10 } }  &Model Acc.      & 73.89\%     & 72.98\%  &  68.69\%  &  65.23\%  & 62.23\%   \\  
			\rowcolor{verylightgray}
			On Cifar10 &Backdoor Acc.    & 9.40\%       & 6.20\%   & 5.80\%   &  4.00\%   &  2.48\%   \\  
			& Running Time     &  6.63        &  3.72     &  2.83      &  2.51     & 2.23 \\
			\bottomrule[0.8pt]
	\end{tabular}}
\end{table}

\begin{table}[H]
	\scriptsize
	\caption{Membership inference attack accuracy after unlearning by OUbL. The results demonstrate that OUbL can effectively reduce the MI accuracy, achieving a significant unlearning performance. @{\color{orange}Reviewer 5Whi}}
	\label{Membership_inf}
	\resizebox{\linewidth}{!}{
		\setlength\tabcolsep{7.5pt}
		\begin{tabular}{c|c|c|c|c|c}
			\toprule[0.8pt]
			\midrule
			Dataset & Original Model & ASR and CSR, 1\% & 2\% & 3\% & 4\% \\
			\midrule
			On MNIST    & 63.86\%     & 53.87\%  &  53.61\%  &  53.02\%  &  52.86\%   \\  
			\rowcolor{verylightgray}
			On CIFAR10    & 77.43\%       & 61.47\%   & 61.30\%   &  61.10\%   &  60.92\%   \\  
			On CelebA     &  58.37\%        &  51.94\%     &  51.32\%     &  51.04\%     &  50.69\%  \\
			\midrule
			\bottomrule[0.8pt]
	\end{tabular}}
\end{table}

 \begin{table}[H]
 	\scriptsize
 	\caption{The detailed running time. The results demonstrate that although we put more computational cost on the user side, it is affordable for users compared to the FL users in BFU. @{\color{purple}Reviewer Ha5f}}
 	\label{detailed_running_time}
 	\resizebox{\linewidth}{!}{
 		\setlength\tabcolsep{7.5pt}
 		\begin{tabular}{c|c|c|c|c|c}
 			\toprule[0.8pt]
 			\midrule
 			Dataset & \makecell[c]{ \makecell[c]{Total running time} \\ \makecell[c]{ of OUbL (second)} }&  \makecell[c]{Unlearning update \\ estimation (User side) } &  \makecell[c]{ Unlearning noise generation \\ (User side) } &  \makecell[c]{Unlearning by incremental \\ learning (Server side) }&  \makecell[c]{Total running time \\of BFU} \\
 			\midrule
 			On MNIST    & 3.92     & 1.06  &  1.45  &  1.41  &  16.03   \\  
 			\rowcolor{verylightgray}
 			On CIFAR10    & 6.64       & 1.02   & 2.10   &  3.52   &  141.26   \\  
 			On CelebA     &  2.26        &  0.72     &  0.83     &  0.71     &  176.86  \\
 			\midrule
 			\bottomrule[0.8pt]
 	\end{tabular}}
 \end{table}

 \begin{table}[H]
	\scriptsize
	\caption{Experimental results on Adult. The task of the Adult dataset is to predict whether an individual's income exceeds \$50,000 per year, which is a binary classification. We first backdoor some samples in Adult by setting the ``education-num'' feature to 2 and changing the corresponding label. The aim of unlearning is to remove the influence of these backdoored samples, and the results are presented in the following table. Since the task on the Adult dataset is a binary task, dropping the backdoor accuracy of around 50\% is similar to the random selection. Our method can effectively degrade the backdoor accuracy to around 50\%, guaranteeing the effectiveness of unlearning. @{\color{cyan} Reviewer Gp18} }
	\label{on_adult}
	\resizebox{\linewidth}{!}{
		\setlength\tabcolsep{7.5pt}
		\begin{tabular}{c|c|c|c|c|c}
			\toprule[0.8pt]
			\midrule
			On Adult & Original & ASR and CSR, 1\%   & 2\% &  3\%&  4\% \\
			\midrule
			Model Acc.    & 85.32\%      & 81.66\%  & 81.69\%   &  79.93\%  & 80.79\%    \\  
			\rowcolor{verylightgray}
			Backdoor Acc.    & 100.00\%        & 54.81\%   & 52.81\%   &  50.02\%    &   49.52\%   \\  
			Running Time     &  15.31        &  0.54     &  1.03     & 1.51      &  1.93   \\
			\midrule
			\bottomrule[0.8pt]
	\end{tabular}}
\end{table}

%In this section, we start by introducing the threat model for unlearning processes in the MLaaS scenario, detailing the abilities of both the ML server and the unlearning users. Then, we introduce the privacy-preserving machine unlearning problem based on the threat model and reformulate it as oblivious unlearning by learning problem.

\section{Scenarios and Threat Model}

%\subsubsection{Machine Unlearning Service Scenarios}

@{\color{blue}Reviewer BZGC}, @{\color{red}Reviewer iCGz}, @{\color{orange}Reviewer 5Whi}, @{\color{magenta}Reviewer EoYb}, @{\color{purple}Reviewer Ha5f},@{\color{cyan} Reviewer Gp18}

\textbf{Machine Unlearning Service Scenarios.}  To facilitate understanding, we introduce the problem in a Machine Learning as a Service (MLaaS) scenario. In the MLaaS setting, there are two key entities: a ML server that trains models as ML services, and users (data owners) who contribute their data for ML model training. In such scenarios, machine unlearning occurs when users realize that some of their previously contributed samples are private and wish to revoke these data contributions from the trained models.  

\textbf{The ML Server's Ability.} We assume the ML server is honest but curious [R1]: while it honestly hosts and provides ML services, including model training and updating, it may still be curious about private information, such as \textbf{unlearned data} and \textbf{unlearning intentions}, if there are other operations. Informing the server of unlearning intentions to customize unlearning operations is considered a privacy threat because it reveals users' unlearning purposes, potentially enabling the server to prepare targeted unlearning attacks [R1,R2]. Therefore, in our setting, we assume the ML server has only the learning algorithm $\mathcal{A}$ and the model with parameters $\theta$ to meet strict privacy requirements. The ML server will not conduct unlearning operations other than training the model using the learning algorithm $\mathcal{A}$ for model updating.   

Moreover, we assume the ML server does not store the original training data and cannot access the erased data, which should not be exposed to the server again due to privacy concerns. This assumption is reasonable in both real-world and privacy-preserving MLaaS scenarios. In real-world applications, vast amounts of data are generated daily, leading to the need of prompt model updates. Consequently, many models are trained using incremental or continual learning techniques [R3,R4]. Therefore, the server does not retain the entire raw data due to its large size [R5,R6]. In privacy-preserving scenarios, the ML server is restricted from directly accessing private training data from users due to privacy concerns [R7,R8].

\textbf{The Users' Ability.} The training data $D$ was collected from all users and was used to train the model $\theta_o$. The unlearning user has the erased data $D_u \subset D$. To estimate the unlearning update as the target for unlearning noise generation in our method, we assume the unlearning user can access the trained model $\theta_o$, which is a common setting even in many privacy-preserving scenarios such as FL. We assume the unlearning user has auxiliary clean examples $D_a$ so that they can synthesize a new dataset based on it with the unlearning noise, replacing the erased data $D_u$ for achieving the unlearning effect with only incremental learning using the synthesized dataset.

\section{Discussion about Distinguishing Benign Unlearning Users and Malicious Users @{\color{red}Reviewer iCGz}}

To distinguish a benign user who wants to delete their data from a malicious user and who wants to upload noisy gradients to sabotage the model performance, we can only propose some possible ways for the server to distinguish these two kinds of users. The most significant difference is the purposes of the unlearning user and the malicious user. Unlearning users want to remove some knowledge of their data from the model, and they also want to preserve the model's utility. Therefore, most clean samples and the auxiliary data they choose are in the same distribution as the genuine samples, and the synthesized noise should not influence the utility of the remaining dataset, as shown in the second objective of Eq.(4). However, the purpose of the malicious user is to sabotage the model performance. Their uploaded data will not be consistent with the genuine samples, so they can degrade model utility. We believe checking the similarity between the uploaded samples and genuine samples would be a possible solution. However, detailed poisoning attacking methods may need different solutions, and the problem is valuable to investigate in future work.

\section{Discussion about Difference between Existing Unlearning Methods @{\color{cyan} Reviewer Gp18}}
Compared with existing representative approximate unlearning methods [R19, R20, R21], our method also has the following differences. Specifically, the key techniques used in [R20] are the Hessian approximation and Fisher information, which is similar to our unlearning update estimation method that is also based on the Hessian matrix. The difference is that we use Hessian-vector products (HVPs) while [R20] uses the Fisher information to improve the efficiency. The HVPs solution is more efficient and more suitable to our scenarios in which the unlearning user cannot access the remaining dataset. [R19] and [R21] are approximate unlearning methods based on techniques called error maximizing. They generate error-maximizing noise for the unlearned samples to remove the influence from the model. One significant advantage of [R19] and [R21] is that they do not require access to the remaining training dataset. Compared with them, we put more effort into designing the method to further hide the unlearning data and the unlearning intentions from the server.

\section{Additional Experiments on the More Practical Black-Box Scenarios @{\color{purple}Reviewer Ha5f}}

To prove the feasibility of our method in the more practical black-box scenarios, we conducted additional experiments on the black-box setting on MNIST and CIFAR10. In this setting, the unlearning user cannot access the server's current model. The unlearning user only knows the type of the model (MLP on MNIST and CNN on CIFAR10 in our experiment), and the user only has the erasing data and the auxiliary data. We set the size of auxiliary data to 1\% of the server-side training data. Other unlearning settings are the same as the main setting in the paper, where we first backdoor the erasing data for model training and aim to unlearn these backdoored erasing data.

With these settings, the unlearning user trains a shadow model ($\theta_s$) with 94.55\% accuracy on MNIST and 42.57\% accuracy on CIFAR10. By contrast, the accuracy of the server's model ($\theta_o$) trained with the entire dataset is 98.74\% on MNIST and 78.80\% on CIFAR10. Since both models are optimized on the erasing dataset, the proposed efficient unlearning update estimation (EUUE) method is effective for simulating the update of the unlearning data based on the shadow model. Hence, we can generate effective noise for the incremental learning data to approach the influence of unlearning. Then, we upload the constructed data to the server side for incremental learning, aiming to achieve the unlearning effect at the same time. We present the results as follows in \Cref{additional_exp_on_black_b}.

\begin{table}[H]
	\scriptsize
	\caption{Additional experiments on the black-box setting. On both datasets, OUbL achieves effective unlearning performance, effectively removing the backdoor influence. The backdoor removal effectiveness in the black-box setting is slightly lower than in the white-box setting. However, the negative impact on the model utility is also mitigated. These experimental results demonstrate the feasibility of OUbL in a more practical scenario, which lets the unlearning user not rely on the assumption of white-box access to the trained model in the federated learning scenarios. @{\color{purple}Reviewer Ha5f}
}
	\label{additional_exp_on_black_b}
	\resizebox{\linewidth}{!}{
		\setlength\tabcolsep{7.5pt}
		\begin{tabular}{c|c|c|c|c|c|c}
			\toprule[0.8pt]
			\midrule
			& Metrics & USR  = 1\%  & 2\%  & 3\% & 4\% & 5\% \\
			\midrule
			\multirow{4}{*}{\makecell[c]{ } }  &Model Acc.(white-box)  & 98.52\%    & 98.55\% &  98.15\%  &  98.19\% &  95.43\%         \\  
			\rowcolor{verylightgray}
			On MNIST  &Model Acc. (black-box)    & 98.26\%    &  98.20\% &   98.31\% &    98.27\%  &  98.54\%     \\  
			& Backdoor Acc. (white-box)     &  9.67\%     & 10.08\%   & 9.83\%   &  10.42\%   &  10.57\%       \\
			\rowcolor{verylightgray}
			& Backdoor Acc. (black-box)     &  12.33\%      &  9.58\%   & 11.67\%    &  10.64\%   &  11.83\%    \\
			\midrule
			\multirow{4}{*}{\makecell[c]{ } }  &Model Acc.(white-box)     & 73.89\%      & 74.57\%   &  74.50\%  &  75.15\% &     75.99\%    \\  
			\rowcolor{verylightgray}
			On Cifar10 &Model Acc. (black-box)    & 76.06\%   & 75.98\%  &   74.93\%   &    75.06\%  &    74.68\%     \\  
			& Backdoor Acc. (white-box)     & 9.40\%       & 7.30\%   &  7.87\%    &    8.70\%  &    7.24\%     \\
			\rowcolor{verylightgray}
			& Backdoor Acc. (black-box)     &  13.20\%      & 10.20\%   &  8.40\%    &   10.25\%   &    8.28\%    \\
			\bottomrule[0.8pt]
	\end{tabular}}
\end{table}

\section{Additional References}

\small{
[R1]. Hu, Hongsheng, et al. "Learn what you want to unlearn: Unlearning inversion attacks against machine unlearning." IEEE Symposium on Security and Privacy (SP) (2024).  

[R2]. Chen, Min, et al. "When machine unlearning jeopardizes privacy." Proceedings of the 2021 ACM SIGSAC conference on computer and communications security. 2021.  

[R3]. Rolnick, David, et al. "Experience replay for continual learning." Advances in neural information processing systems 32 (2019).  

[R4]. Lopez-Paz, David, and Marc'Aurelio Ranzato. "Gradient episodic memory for continual learning." Advances in neural information processing systems 30 (2017).  

[R5]. Wu, Yue, et al. "Large scale incremental learning." Proceedings of the IEEE/CVF conference on computer vision and pattern recognition. 2019.  

[R6]. Wang, Zifeng, et al. "Learning to prompt for continual learning." Proceedings of the IEEE/CVF conference on computer vision and pattern recognition. 2022.  

[R7]. Naseri, Mohammad, Jamie Hayes, and Emiliano De Cristofaro. "Local and central differential privacy for robustness and privacy in federated learning." NDSS (2022).  

[R8]. Bonawitz, Keith, et al. "Practical secure aggregation for privacy-preserving machine learning." proceedings of the 2017 ACM SIGSAC Conference on Computer and Communications Security. 2017.  

[R9]. Gao, Xiangshan, et al. "Verifi: Towards verifiable federated unlearning." IEEE Transactions on Dependable and Secure Computing (2024).

[R10]. Guo, Xintong, et al. "Fast: Adopting federated unlearning to eliminating malicious terminals at server side." IEEE Transactions on Network Science and Engineering (2023).

[R11]. Zhu, Ligeng, Zhijian Liu, and Song Han. "Deep leakage from gradients." Advances in neural information processing systems 32 (2019).

[R12]. Kurmanji, M., Triantafillou, P., Hayes, J. and Triantafillou, E., 2024. Towards unbounded machine unlearning.Advances in neural information processing systems, 36.

[R13]. Chen, Min, et al. "When machine unlearning jeopardizes privacy." Proceedings of the 2021 ACM SIGSAC conference on computer and communications security. 2021.

[R14]. Hu, Hongsheng, et al. "Membership inference via backdooring." IJCAI (2022).  

[R15]. Bertram, Theo, et al. "Five years of the right to be forgotten." Proceedings of the 2019 ACM SIGSAC Conference on Computer and Communications Security. 2019.  

[R16]. Oh, Seong Joon, Bernt Schiele, and Mario Fritz. "Towards reverse-engineering black-box neural networks." Explainable AI: interpreting, explaining and visualizing deep learning (2019): 121-144.  

[R17]. Salem, Ahmed, et al. "{Updates-Leak}: Data set inference and reconstruction attacks in online learning." 29th USENIX security symposium (USENIX Security 20). 2020.  

[R18]. Wang, Binghui, and Neil Zhenqiang Gong. "Stealing hyperparameters in machine learning." 2018 IEEE symposium on security and privacy (SP). IEEE, 2018.  

[R19] Chundawat, Vikram S., et al. "Zero-shot machine unlearning." IEEE Transactions on Information Forensics andSecurity 18 (2023): 2345-2354.  

[R20] Golatkar, Aditya, Alessandro Achille, and Stefano Soatto. "Eternal sunshine of the spotless net: Selective forgettingin deep networks." Proceedings of the IEEE/CVF Conference on Computer Vision and Pattern Recognition. 2020.  

[R21] Tarun, Ayush K., et al. "Fast yet effective machine unlearning." IEEE Transactions on Neural Networks and LearningSystems (2023).  

}
