# Supplementary material for: GeoIB: Geometry-Aware Information Bottleneck via Statistical-Manifold Compression
Source: arXiv:2602.03906 source file (2026-02-03)
Supplement: Supplementary file 3 [file appendix3.tex]

\subsection{Sequential Time Analysis of Sharding}
\label{appendix:time_sharding_sequential}

\noindent{\em Proof:} \\
\noindent\emph{1. Assumption:} At each step and for all shards, the probability that an unlearning request affects that specific shard is approximately equal to $\frac{1}{S}$. The intuition is as follows: if many points from a specific shard are deleted as unlearning occurs, the number of such (unlearnable) points decreases and they are therefore less likely to be deleted. Conversely, if few points from that shard are deleted, the proportion of those points increases as points from other shards are deleted. Thus, they become more likely to be deleted. 

\noindent\emph{2. Intuition:} The size of the shard that is affected by the first request is always $\frac{N}{S}$. For the second request, it can be either $\frac{N}{S}$ with probability $\left(1 - \frac{1}{S}\right)$ if the request does not affect the same shard or $\left(\frac{N}{S} - 1\right)$ with probability $\frac{1}{S}$ if it does. For the third request it can be $\frac{N}{S}$, $\left(\frac{N}{S} - 1\right)$, or $\left(\frac{N}{S} - 2\right)$. Note that there are two ways to get $\left(\frac{N}{S} - 1\right)$: either from a shard that had $\left(\frac{N}{S} - 1\right)$ point before the previous request and that was not affected by it, or from a shard that had $\frac{N}{S}$ points before the previous request and that was affected by it.

\noindent\emph{3. Size of the retraining set:} To model this behavior, we define the event $E_{i,j}$ as
the $i^{th}$ request received landing on shard $s$ containing $\frac{N}{S} - j$ points, with $j \in \{0,\dots,i - 1\}$. The associated cost is $\frac{N}{S} - j - 1$.

\noindent\emph{4. Associated probability:} The probability of $E_{i,j}$ given a configuration of the $j$ requests, \ie which specific subset of the $i-1$ requests corresponds to those that landed on $s$, is $\left(\frac{1}{S}\right)^j\left(1 - \frac{1}{S}\right)^{i-1-j}$. The first term of the product means that shard $s$ was affected $j$ times, and the second term means that another shard (but not $s$) was affected $i - 1 - j$ times. However, there are ${i - 1 \choose j}$ possible configurations of the $j$ requests that landed on shard $s$. Thus the probability of $E_{i,j}$ is ${i-1 \choose j}\left(\frac{1}{S}\right)^j\left(1-\frac{1}{S}\right)^{i-j-1}$.

\noindent\emph{5. Expected cost:} The expected cost of the $i^{th}$ unlearning request can be decomposed on the family of events $(E_{i,j})_j$ (with only $j$ varying between $0$ and $i-1$) that partitions the universe of possible outcomes:
\begin{equation}\mathbb{E}[C_i] =\sum_{j=0}^{i-1}{{i-1 \choose j}\left(\frac{1}{S}\right)^j\left(1-\frac{1}{S}\right)^{i-j-1} \left(\frac{N}{S} - 1 - j\right)}\end{equation}

To obtain the total cost, we sum the costs of all unlearning requests, which is to say we sum over $i$ between $1$ and $K$.

{\small
\begin{equation}\begin{aligned}
\mathbb{E}[C] &=\sum_{i=1}^{K}\sum_{j=0}^{i-1}{{i-1 \choose j}\left(\frac{1}{S}\right)^j\left(1-\frac{1}{S}\right)^{i-j-1} \left(\frac{N}{S} - 1 - j\right)}\\
&=\sum_{i=1}^{K}{\left(\frac{N}{S} - 1\right)\sum_{j=0}^{i-1}{{i-1 \choose j}\left(\frac{1}{S}\right)^j\left(1-\frac{1}{S}\right)^{i-j-1}}}\\
&-\sum_{i=1}^{K}\sum_{j=0}^{i-1}{j{i-1 \choose j}\left(\frac{1}{S}\right)^j\left(1-\frac{1}{S}\right)^{i-j-1}}
\end{aligned}\end{equation}
}

We can use the fact that $j{i-1 \choose j} = (i-1){i-2 \choose j-1}$ and apply the binomial theorem to both inner sums after reindexing the second inner sum.

{\small
\begin{equation}\begin{aligned}
\mathbb{E}[C] &= \left(\frac{N}{S} - 1\right)K - \sum_{i=1}^{K}{\frac{i-1}{S}}\\
\end{aligned}\end{equation}
}
