# Supplementary material for: GeoIB: Geometry-Aware Information Bottleneck via Statistical-Manifold Compression
Source: arXiv:2602.03906 source file (2026-02-03)
Supplement: Supplementary file 8 [file appendix8.tex]

\subsection{Impact of aggregation strategy}
\label{appendix:aggregation_strategy}

\new{Due to the nature of SISA, we need to aggregate the predictions of different models. Here we tested 2 aggregation strategies on 4 datasets respectively, the results can be found in Figures~\ref{fig:aggregation_strategy1} and~\ref{fig:aggregation_strategy2}.}

\begin{figure}[H]
\centering
\subfloat[{{\small SVHN}}]{\label{fig:svhn_aggregation}{\includegraphics[width=0.5\linewidth]{Figures/svhn_aggregation.pdf}}  } 
\subfloat[{{\small Purchase}}]{\label{fig:purchase_aggregation}{\includegraphics[width=0.5\linewidth]{Figures/purchase_aggregation.pdf}}  } 
\caption{\small \new{We explore the effect of aggregating labels versus aggregation prediction vectors, on Purchase and SVHN. It can be seen that on these easy datasets, changing aggregation strategy does not influence performance of the models significantly.}\vspace{-5mm}} 
\label{fig:aggregation_strategy1}
\end{figure}

\begin{figure}[H]
\centering
\subfloat[{{\small Imagenet}}]{\label{fig:imagenet_aggregation}{\includegraphics[width=0.5\linewidth]{Figures/imagenet_aggregation_top5.pdf}}  } 
\subfloat[{{\small Mini-Imagenet}}]{\label{fig:miniimagenet_aggregation}{\includegraphics[width=0.5\linewidth]{Figures/miniimagenet_aggregation_top5.pdf}}  } 
\caption{\small \new{We explore the effect of aggregating labels versus aggregation prediction vectors, on Mini-ImageNet and ImageNet. It can be seen that on these hard tasks such as classifying high-resolution images, a good aggregation strategy is able to help recover more accuracy.}\vspace{-5mm}} 
\label{fig:aggregation_strategy2}
\end{figure}
